# Supplementary material for: Design Rules for Interconnects Based on Graphene Nanoribbon Junctions
Source: arXiv:2402.17186 ancillary file (2024-02-27)
Supplement: Supplementary file 1 [file Supplementary.pdf]

# Supplementary Material for: "Design Rules for Interconnects Based on Graphene Nanoribbon Junctions"

Kristiāns Čerņevičs and Oleg V. Yazyev

*Institute of Physics, Ecole Polytechnique Fédérale de Lausanne (EPFL), CH-1015, Switzerland*

## SUPPLEMENTARY FIGURES

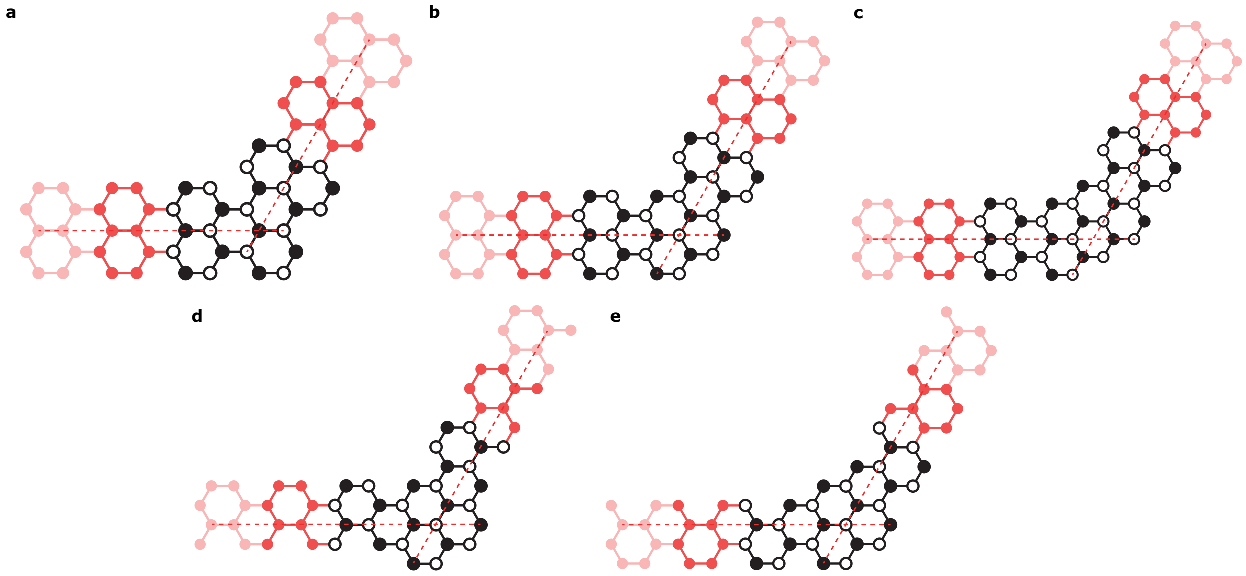


FIG. 1. Definition of 3 classes of angled junctions. The axes of AGNR leads ($N = 5$ in this illustration) intersect (a) the atomic position in one of the sublattices marked with black (intersection point $IP_A$), (b) in the complementary sublattice marked with white ($IP_B$) or (c) in the empty (center of a hexagon) position ($IP_C$). The intersection point $IP$ can be controlled by adjusting the distance between the leads. For leads with even number of atoms across the width there are two possibilities for attaching the leads for each of the classes, hence doubling the number of structures. The AGNR ($N = 4$) leads attached in the (d) *up* configuration and (e) *down* configuration. The distinctions *up* and *down* correspond to the aligned edge with respect of the ($N$+1)-AGNR (in this case panel (b)).

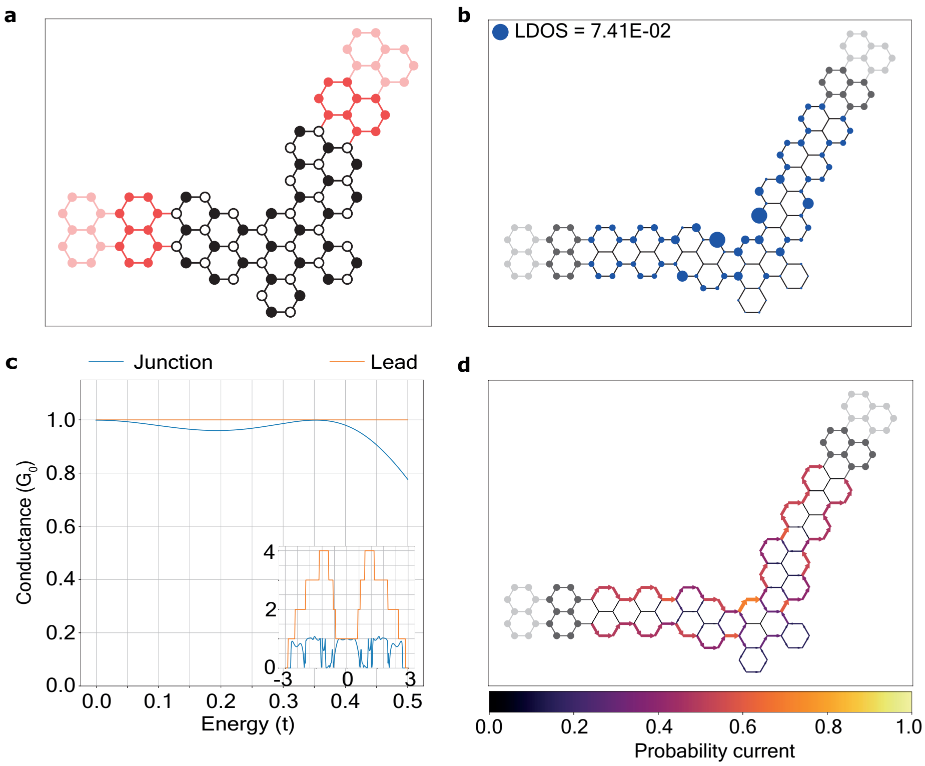


FIG. 2. (a) Atomic structure of a selected 5-AGNR 120° junction with mixed-edge scattering centre. (b) LDOS of the junction at $E = 0$. (c) Conductance profile of the junction in the $0 \leq E \leq 0.5t$ energy range and the full conductance profile shown in the inset. (d) Local current across the junction at $E = 0$.

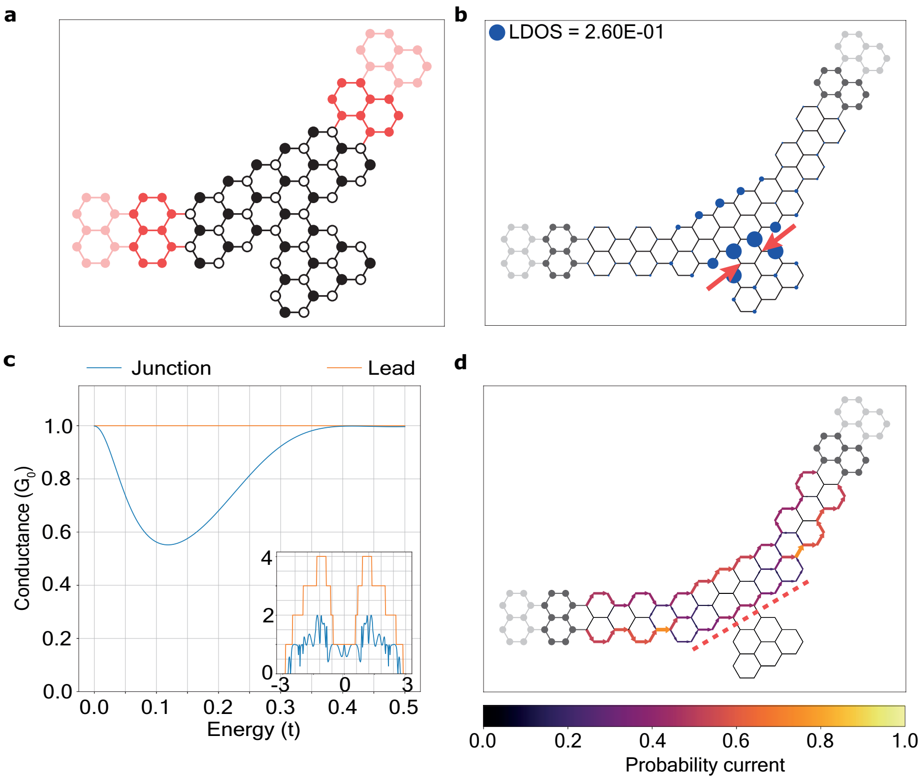


FIG. 3. (a) Atomic structure of a selected 5-AGNR 120° junction with sublattice imbalance $\delta N = -2$. (b) LDOS of the junction at $E = 0$. (c) Conductance profile of the selected junction in the $0 \leq E \leq 0.5t$ energy range and the full conductance profile shown in the inset. (d) Local current of the junction at $E = 0$. We note that the lower triangular fragment is decoupled from the rest of the junction as the atoms marked with the red arrows in (b) show no electron density. Hence, the local current in (d) can only be observed in the region above the red dashed line, where sublattice imbalance of $\delta N = -1$ is preserved.

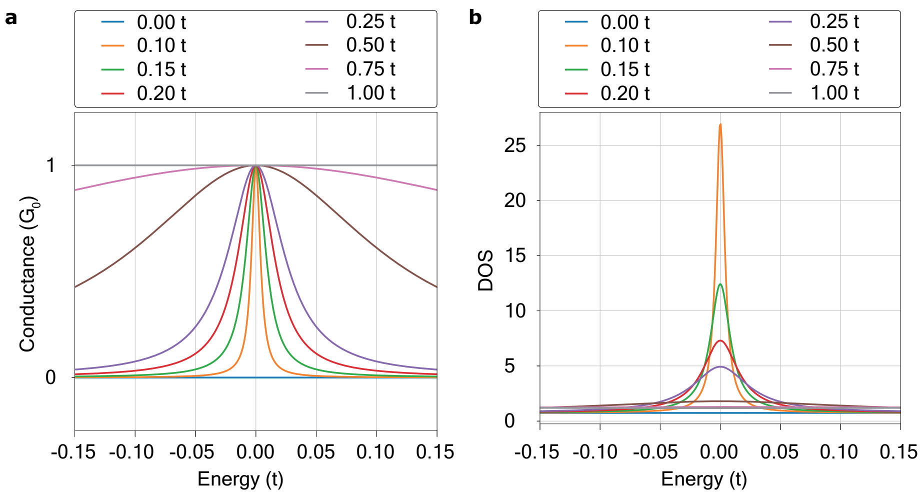


FIG. 4. Transport through a zero-energy state. Evolution of (a) conductance and (b) DOS peak near $E = 0$ upon changing the strength $t$ of the coupling to the leads.

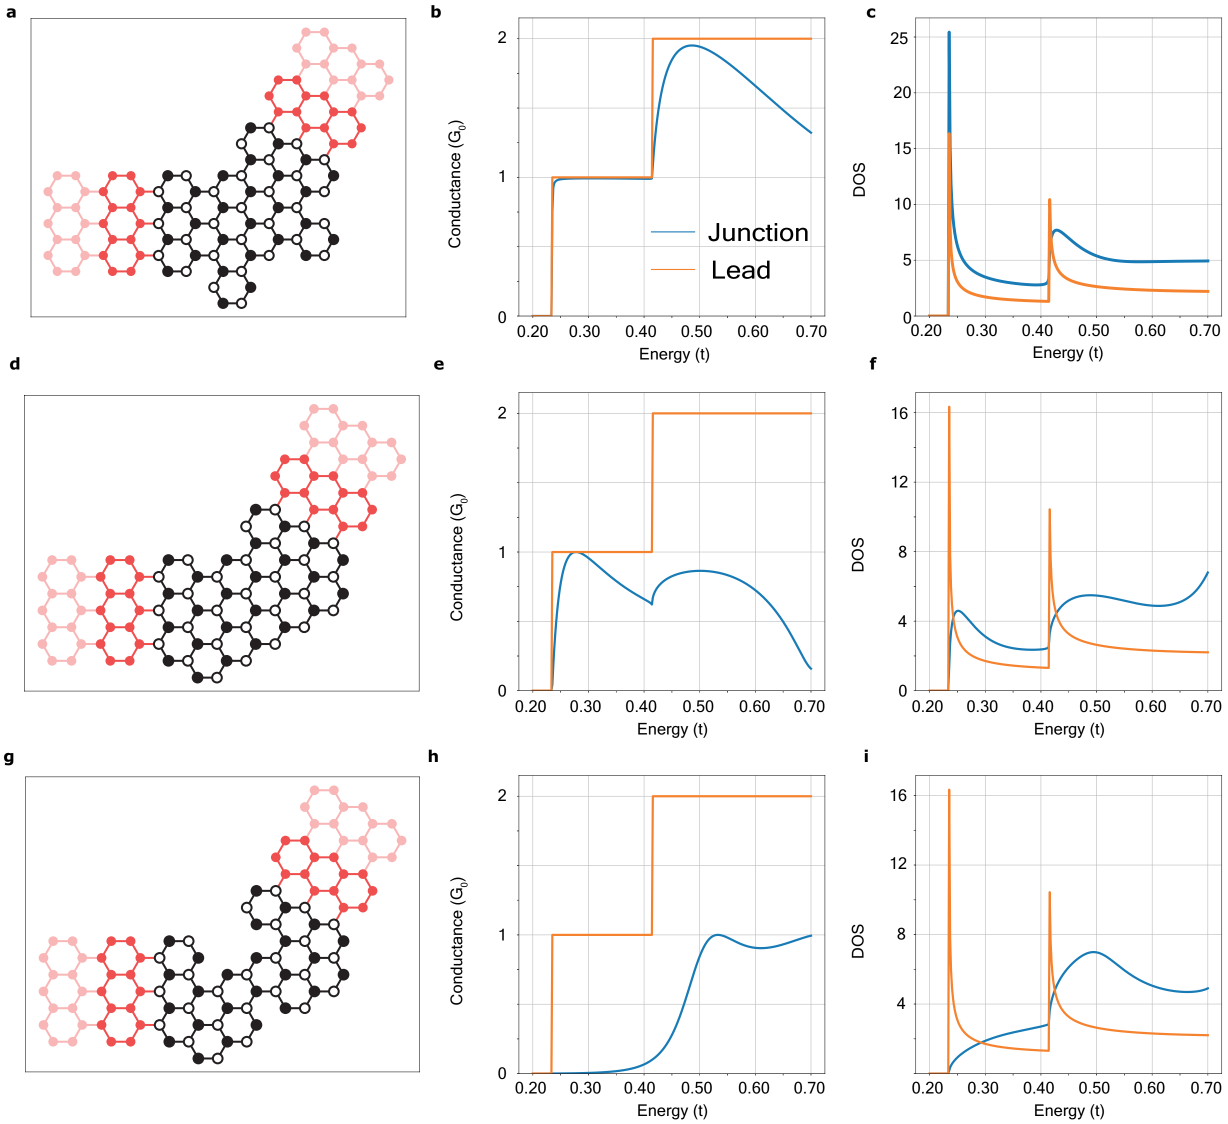


FIG. 5. (a) Atomic structure of a 7-AGNR 120° junction with $\tau = 1$. (b) Conductance profile and (c) DOS of the junction in the $0 \leq E \leq 0.5t$ energy range. (d) Atomic structure of a 7-AGNR 120° junction with $\tau = 0.78$. (e) Conductance profile and (f) DOS of the junction in the $0 \leq E \leq 0.5t$ energy range. (g) Atomic structure of a 7-AGNR 120° junction with $\tau = 0$. (h) Conductance profile and (i) DOS of the junction in the $0 \leq E \leq 0.5t$ energy range.

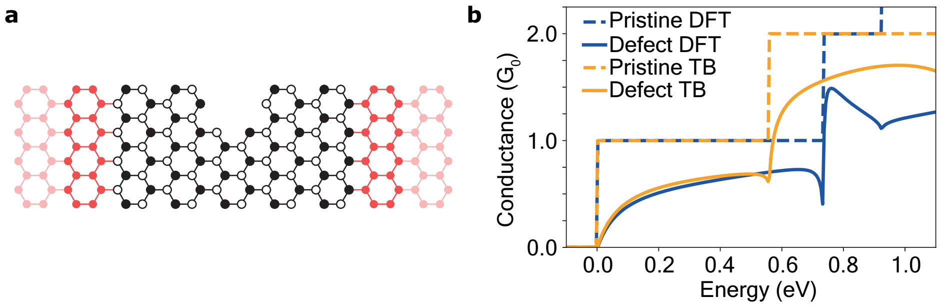


FIG. 6. Comparison of DFT and nearest-neighbour TB calculations. (a) Atomic structure of a 9-AGNR with a "bite" defect investigated in our previous work [1] and (b) calculated conductance for pristine and defective cases with DFT and TB models. Conductance band edge is set to $E = 0$.

## APPENDIX: BINARY CONDUCTANCE ACROSS METALLIC 120° JUNCTIONS

Below we discuss the origin of binary conductance in metallic 120° AGNR junctions. We will demonstrate how in the case of no sublattice imbalance the structure of Hamiltonian matrix $H_D$ results in $T = 0$, and hence $G = 0$ at $E = 0$. We will be representing our $H_D$ as a block matrix, where zero blocks correspond to the two sublattices and the only hopping terms are between atoms in the complementary sublattices

$$H_D = \left[\begin{array}{c|c} 0 & t_{ab} \\ \hline t_{ab}^{\dagger} & 0 \end{array}\right]. \tag{1}$$

Next, as discussed in the main text, we recall that the self-energy of the leads is acting only on one sublattice for the 120° 2-terminal junctions

$$H_{eff}(E) = H_D + \Sigma_L(E) + \Sigma_R(E) = \left[\begin{array}{c|c} 0 & t_{ab} \\ \hline t_{ab}^{\dagger} & 0 \end{array}\right] + \left[\begin{array}{c|c} \Sigma_L(E) + \Sigma_R(E) & 0 \\ \hline 0 & 0 \end{array}\right]. \tag{2}$$

We continue by expressing the Green's function as a block matrix

$$G(0) = ((i\eta)I_D - H_{eff})^{-1} = \left[\begin{array}{c|c} i\eta - \Sigma_{L+R} & -t_{ab} \\ \hline -t_{ab}^{\dagger} & i\eta \end{array}\right]^{-1} = \left[\begin{array}{c|c} G_a & G_b \\ \hline G_c & G_d \end{array}\right], \tag{3}$$

where we introduce the subscripts to denote blocks $a, b, c$ and $d$ in the matrix. Remembering that only one sublattice is attached to the leads, the block matrix $\Gamma_{L(R)}$ is similarly expressed as

$$\Gamma_{L(R)} = \left[\begin{array}{c|c} \Gamma_{L_a(R_a)} & 0 \\ \hline 0 & 0 \end{array}\right]. \tag{4}$$

As the transmission across the junction is obtained by taking the trace of the matrix product in Eq. 5, we refer to this product as $F$ for clarity

$$T(E) = Tr[F] = Tr[F_1 F_2] = Tr[\Gamma_L G \Gamma_R G^{\dagger}], \tag{5}$$

where we also assign $F_1 = \Gamma_L G$ and $F_2 = \Gamma_L G^{\dagger}$. Now, we are only interested in block $G_a$ as the final matrix $F$ can be expressed as block multiplications:

$$F = \Gamma_L G \Gamma_R G^{\dagger} = \left[\begin{array}{c|c} \Gamma_{L_a} G_a \Gamma_{R_a} G_a^{\dagger} & \Gamma_{L_a} G_a \Gamma_{R_a} G_b^{\dagger} \\ \hline 0 & 0 \end{array}\right] = \left[\begin{array}{c|c} F_a & F_b \\ \hline 0 & 0 \end{array}\right], \tag{6}$$

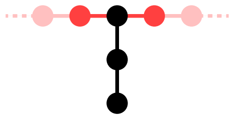

FIG. 7. One-dimensional chain model with 3-site scattering region.

where indices $a$ and $b$ once again refer to the corresponding blocks of the matrix. We also note that taking the trace of $F$ will only involve the block $F_a$. Therefore, showing that the block $G_a$ is zero will imply that the block $F_a$ is also zero, finally leading to $T = 0$. Block matrix inversion is carried out from Eq. 3 to obtain $G_a$

$$G_a = ((i\eta - \Sigma_{L+R}) - (-t_{ab}\frac{I}{i\eta}(-t_{ab}^{\dagger})))^{-1}. \tag{7}$$

In the limit of $\eta \to 0$ we see that block $G_a$ approaches 0 as well.

Further, we can show analytically perfect transmission $T = 1$ (and hence $G = 1$) at $E = 0$ by considering a simplified model system with sublattice imbalance. The model is a one-dimensional chain with the scattering region consisting of 3 sites shown in Fig. 7. Note that this system inherits the discussed properties of more complex systems such the 120° angled GNR junctions discussed in our work. All energy-dependent variables are calculated for $E = 0$.

We will start by transforming the basis of our matrices as ultimately we are interested in the trace of matrix product $F$ and the trace is invariant under the change of basis. As the new basis we will choose the eigenvectors of $H_D$; the $H_D$ is then transformed to diagonal matrix $\tilde{H}_D$ with the trace of 0 as the eigenvalues are pairwise symmetric around 0.

$$H_D = \begin{bmatrix} 0 & 0 & t \\ 0 & 0 & t \\ t & t & 0 \end{bmatrix} \tag{8}$$

$$P^{-1}H_D P = \tilde{H}_D \begin{bmatrix} \sqrt{2}t & 0 & 0 \\ 0 & 0 & 0 \\ 0 & 0 & -\sqrt{2}t \end{bmatrix} \tag{9}$$

$$P = \begin{bmatrix} \frac{1}{\sqrt{2}} & -1 & \frac{-1}{\sqrt{2}} \\ \frac{1}{\sqrt{2}} & 1 & \frac{-1}{\sqrt{2}} \\ 1 & 0 & 1 \end{bmatrix} \tag{10}$$

Similarly, we transform the self-energy energy matrix $\Sigma_{L(R)}$ in the new basis.

$$\Sigma_{L(R)} = \begin{bmatrix} it & 0 & 0 \\ 0 & 0 & 0 \\ 0 & 0 & 0 \end{bmatrix} \tag{11}$$

$$\tilde{\Sigma}_{L(R)} = \begin{bmatrix} \frac{ti}{4} & \frac{t\sqrt{2}i}{4} & \frac{-ti}{4} \\ \frac{t\sqrt{2}i}{4} & \frac{ti}{2} & \frac{-t\sqrt{2}i}{4} \\ \frac{-ti}{4} & \frac{-t\sqrt{2}i}{4} & \frac{ti}{4} \end{bmatrix} \tag{12}$$

We now obtain the Green's function and we notice that the real part of the trace is zero, hence showing that the symmetry along the diagonal is preserved.

$$\tilde{G} = \begin{bmatrix} \frac{1}{\sqrt{2}t} & \frac{-1}{2t} & 0 \\ \frac{-1}{2t} & \frac{i}{t} & \frac{-1}{2t} \\ 0 & \frac{-1}{2t} & \frac{-1}{\sqrt{2}t} \end{bmatrix} \tag{13}$$

Further, we also show the broadening $\tilde{\Gamma}_{L(R)}$, where one can notice that the matrix rows and columns have a property similar to the previously mentioned diagonal symmetry, where the elements in the same row (column) have a pair with an opposite sign except for the element associated with the 0 energy state. For example, in the second row (column), this element is $-t$, while in the other cases it is $\frac{(-)t}{\sqrt{2}}$.

$$\tilde{\Gamma}_{L,R} = \begin{bmatrix} \frac{-t}{2} & \frac{-t}{\sqrt{2}} & \frac{t}{2} \\ \frac{-t}{\sqrt{2}} & -t & \frac{t}{\sqrt{2}} \\ \frac{t}{2} & \frac{t}{\sqrt{2}} & \frac{-t}{2} \end{bmatrix} \tag{14}$$

Finally, we show the matrix $F$ and the corresponding matrices $F_1$ and $F_2$ that have the aforementioned diagonal pairwise symmetry. Although in our specific case these elements are 0, more complex geometries will yield non-zero values. In the general case, when multiplying $F_1$ and $F_2$, only the elements in the row and column associated with the 0 energy state (second row and column) will give non-vanishing values in final matrix $F$. We notice that the rows of $F_1$ and $F_2$ contain pairs of values of the same sign, while columns contain the pairs of values with opposite signs. For example, we show that multiplying row 2 with column 2, to obtain the central element of the matrix $F$ will result in only one non-vanishing term $-i \times i$, which is exactly 1. We associate this element with the 0 energy state.

$$F = F_1 F_2 = \begin{bmatrix} 0 & \frac{-i}{\sqrt{2}} & 0 \\ 0 & -i & 0 \\ 0 & \frac{i}{\sqrt{2}} & 0 \end{bmatrix} \cdot \begin{bmatrix} 0 & \frac{i}{\sqrt{2}} & 0 \\ 0 & i & 0 \\ 0 & \frac{-i}{\sqrt{2}} & 0 \end{bmatrix} = \begin{bmatrix} 0 & \frac{1}{\sqrt{2}} & 0 \\ 0 & 1 & 0 \\ 0 & \frac{-1}{\sqrt{2}} & 0 \end{bmatrix} \tag{15}$$

We note that taking the trace of $F$ with more complex system shows that other diagonal terms will cancel out as the final matrix $F$ keeps the diagonal pairwise symmetry. Hence, for junctions without sublattice imbalance, the trace of $F$ is 0 due to the opposite sign contributions from the energy states. However, for 120° GNR junctions with sublattice imbalance and an eigenvalue of 0, we will see a contribution to transmission in the final matrix $F$ from the zero energy state. We have shown this diagonal value to be exactly 1, hence indicating that the zero-energy state is responsible for the resonant transmission.

---

[1] M. Pizzochero, K. Čerņevičs, G. B. Barin, S. Wang, P. Ruffieux, R. Fasel, and O. V. Yazyev, Quantum electronic transport across 'bite' defects in graphene nanoribbons, 2D Mater. **8**, 035025 (2021).
